# Supplementary material for: Onset of stripe order in classical fluids: Lessons from lattice-gas mixtures
Source: arXiv:2601.14082 ancillary file (2026-01-20)
Supplement: Supplementary file 1 [file supplementary_material.pdf]

**Supplementary Information for**

# Onset of Stripe Order in Classical Fluids: Lessons from Lattice-Gas Mixtures

by Gabriele Costa and Santi Prestipino

---

In this document, we collect graphical information relative to all the particular lattice-gas mixtures analyzed in our paper (red and yellow symbols represent species-1 and species-2 particles, respectively; blue symbols are empty sites). While most cases concern symmetric mixtures under the constraint $\mu_1 = \mu_2$, we have also examined a few non-symmetric mixtures (still for $\mu_1 = \mu_2$) and examples of equimolar mixtures.
The cases are numbered progressively, as in Tables I and II of the main text.

In addition to the equation of state $N(\mu)$, computed for a couple of temperatures, for each case we show a few representative low-temperature patterns and, occasionally, some two-phase coexistence states.

---

## Contents

**1. Symmetric Mixtures** .................... **2**
**2. Asymmetric Mixtures** .................... **23**
**3. Equimolar Mixtures** .................... **27**

# 1. Symmetric Mixtures

1. $U_{\mathrm{AA}} = U_{\mathrm{BB}} = (0,0,0)$, $U_{\mathrm{AB}} = (1,0,0)$

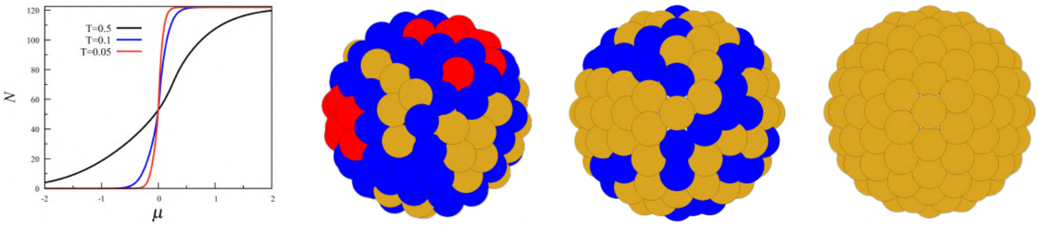


$N = 50$ $N = 80$ $N = 122$

2. $U_{\mathrm{AA}} = U_{\mathrm{BB}} = (0,0,0)$, $U_{\mathrm{AB}} = (1,1,0)$

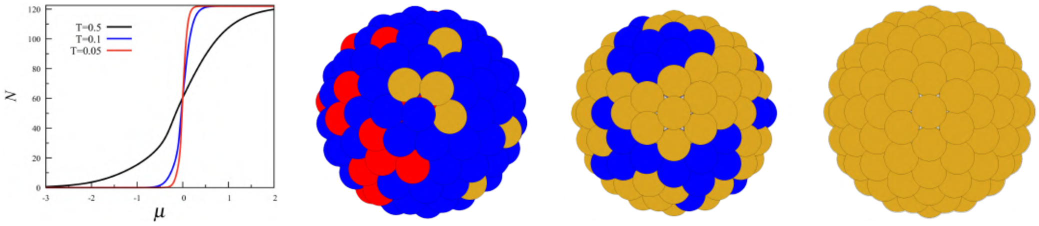


$N = 30$ $N = 80$ $N = 122$

3. $U_{\mathrm{AA}} = U_{\mathrm{BB}} = (1,0,0)$, $U_{\mathrm{AB}} = (0,0,0)$

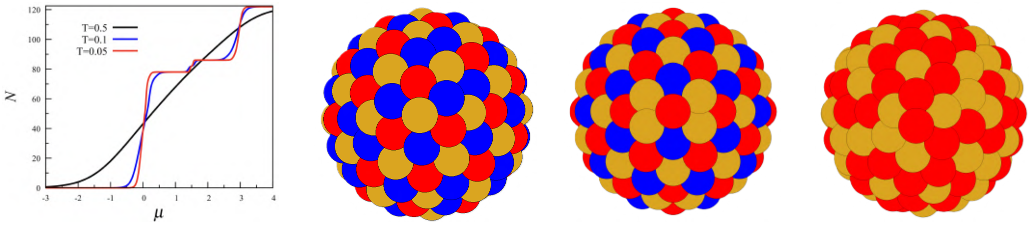


$N = 78$ $N = 86$ $N = 122$

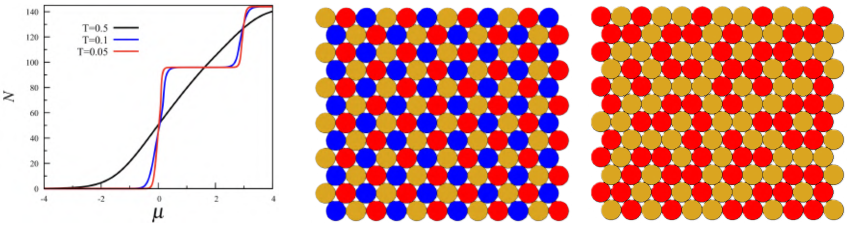


$N = 96$ $N = 144$

4. $U_{\mathrm{AA}} = U_{\mathrm{BB}} = (1, 1, 0)$, $U_{\mathrm{AB}} = (0, 0, 0)$

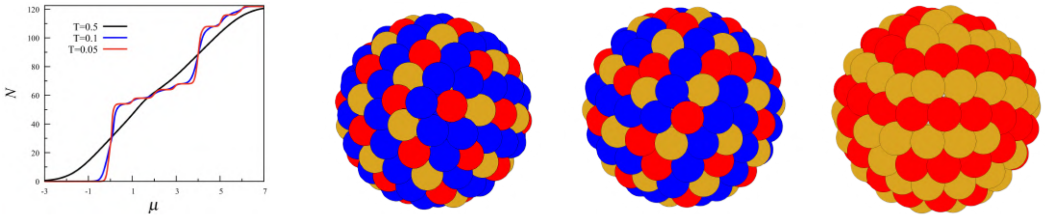


$N = 58$ $N = 64$ $N = 122$

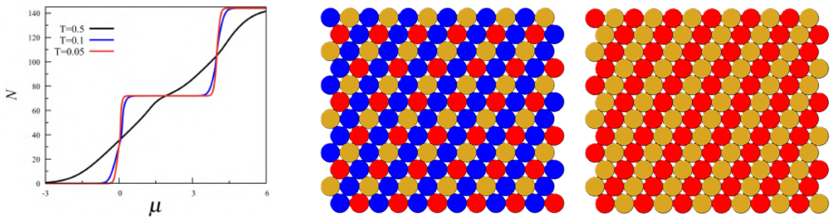


$N = 72$ $N = 144$

5. $U_{\mathrm{AA}} = U_{\mathrm{BB}} = (1, 1, 1)$, $U_{\mathrm{AB}} = (0, 0, 0)$

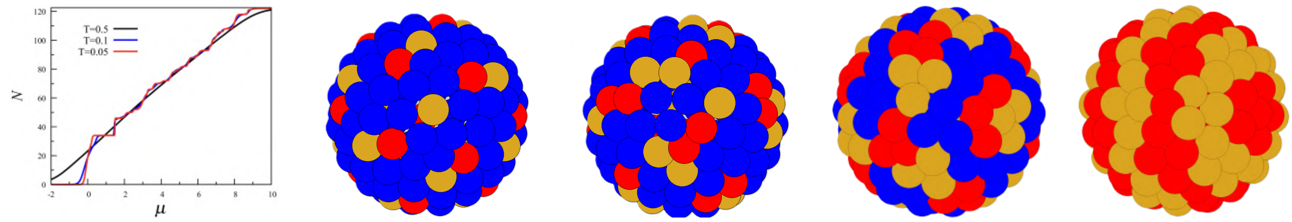


$N = 34$ $N = 50$ $N = 72$ $N = 122$

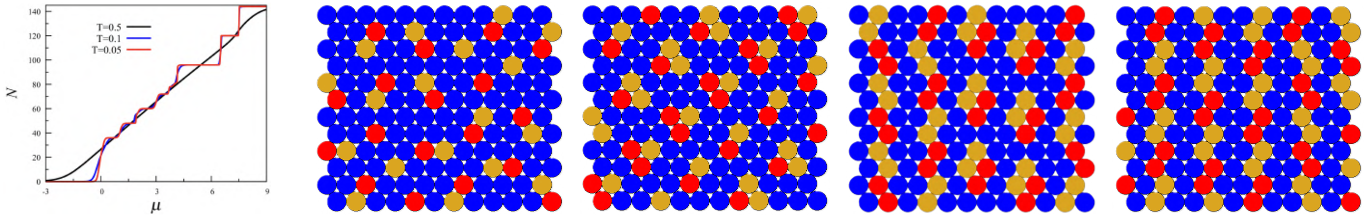


$N = 36$ $N = 48$ $N = 60$ $N = 60$

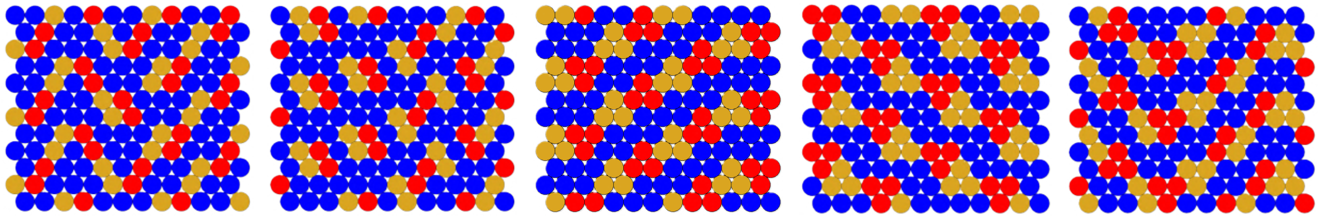

$N = 60$ $N = 60$ $N = 72$ $N = 72$ $N = 72$

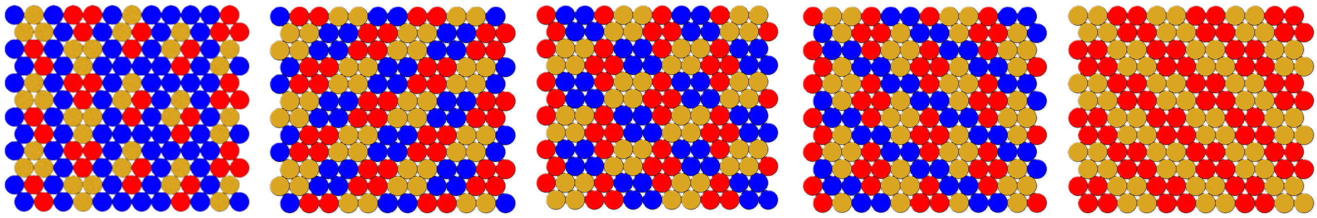

$N = 72$ $N = 96$ $N = 96$ $N = 96$ $N = 144$

6. $U_{\mathrm{AA}} = U_{\mathrm{BB}} = (0, 0, 0)$, $U_{\mathrm{AB}} = (-1, 0, 0)$

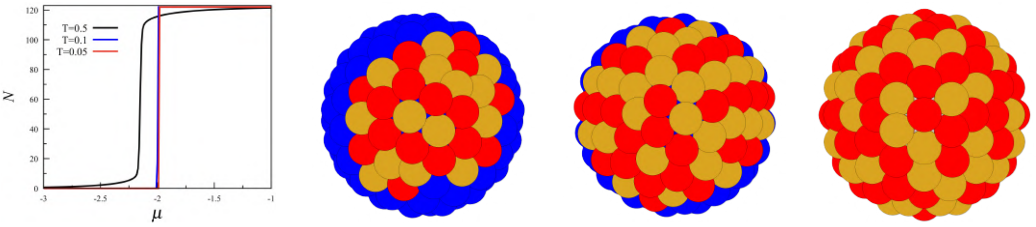


$N = 30$ $N = 50$ $N = 122$

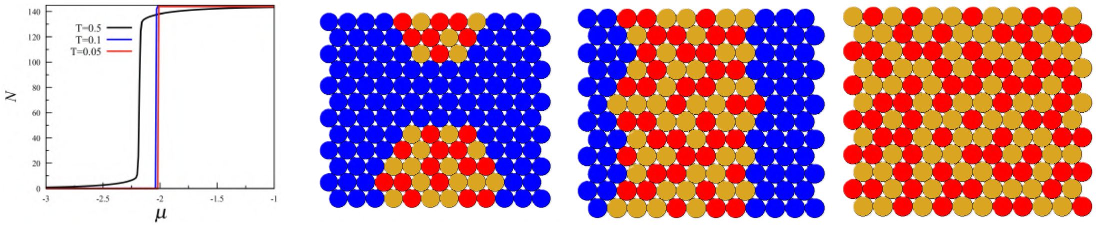


$N = 40$ $N = 80$ $N = 144$

7. $U_{\mathrm{AA}} = U_{\mathrm{BB}} = (0, 0, 0)$, $U_{\mathrm{AB}} = (-1, -1, 0)$

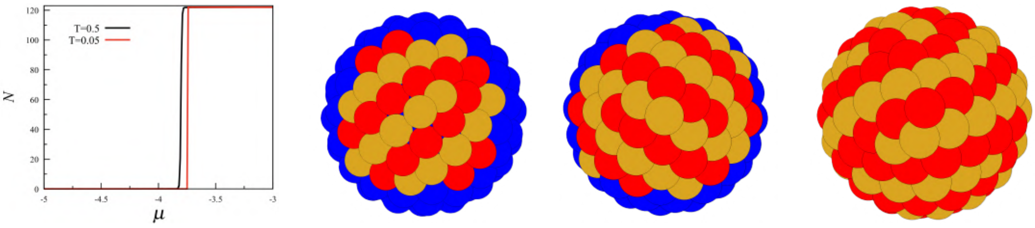


$N = 30$ $N = 40$ $N = 122$

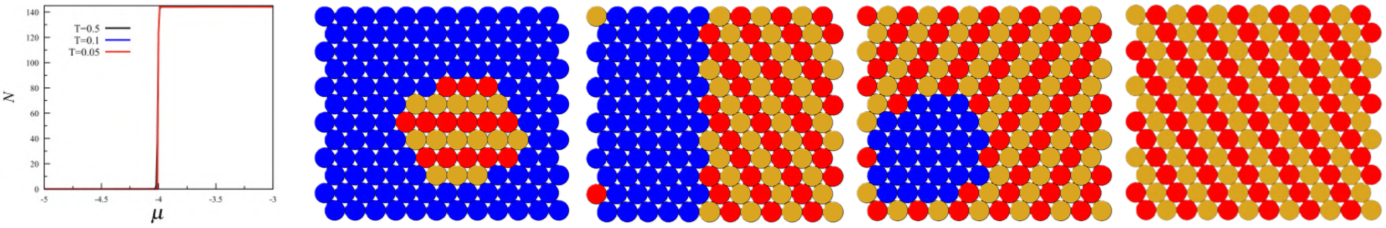


$N = 28$ $N = 80$ $N = 115$ $N = 144$

8. $U_{\mathrm{AA}} = U_{\mathrm{BB}} = (0, 0, 0)$, $U_{\mathrm{AB}} = (-1, -1, -1)$

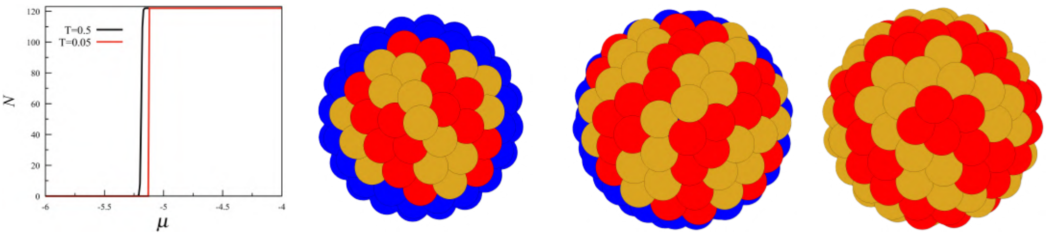


$N = 30$ $N = 50$ $N = 122$

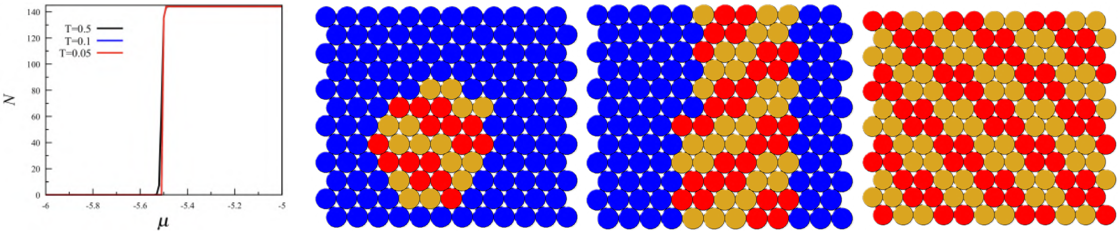


$N = 30$ $N = 60$ $N = 44$

9. $U_{\mathrm{AA}} = U_{\mathrm{BB}} = (0, 0, 0)$, $U_{\mathrm{AB}} = (1, -1, 0)$

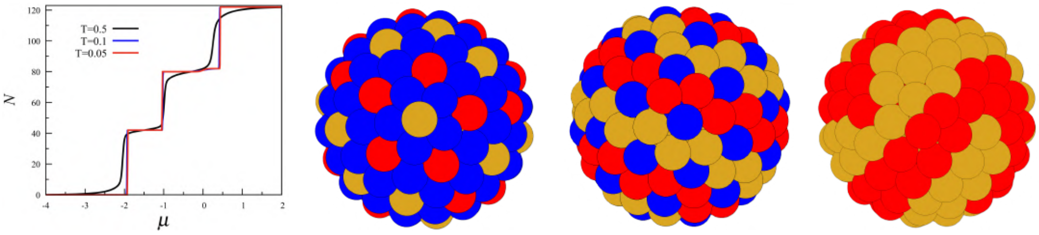


$N = 42$ $N = 80$ $N = 122$

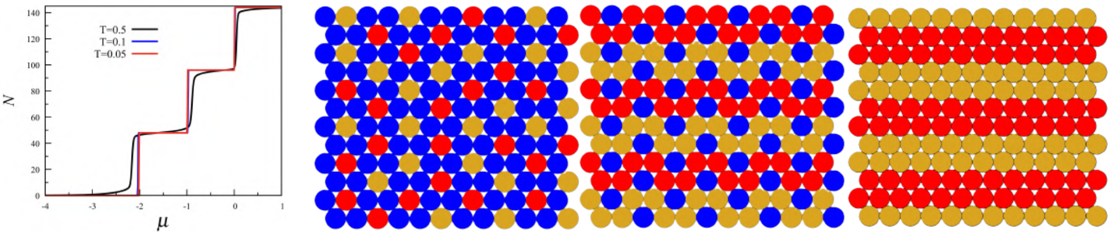


$N = 48$ $N = 96$ $N = 144$

10. $U_{\rm AA} = U_{\rm BB} = (0, 0, 0)$, $U_{\rm AB} = (1, 0, -1)$

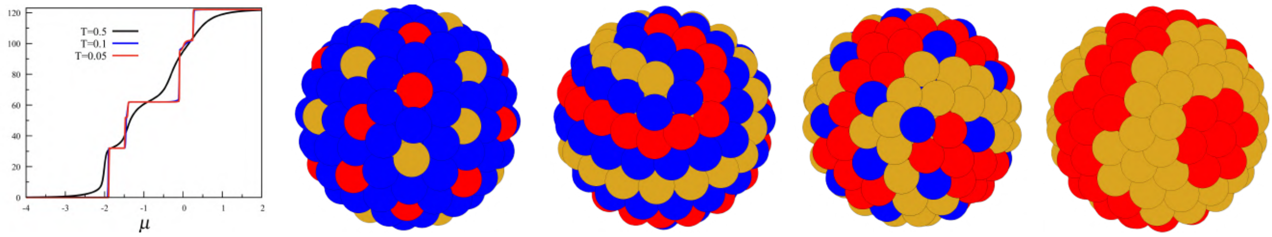


$N = 32$ $N = 62$ $N = 96$ $N = 122$

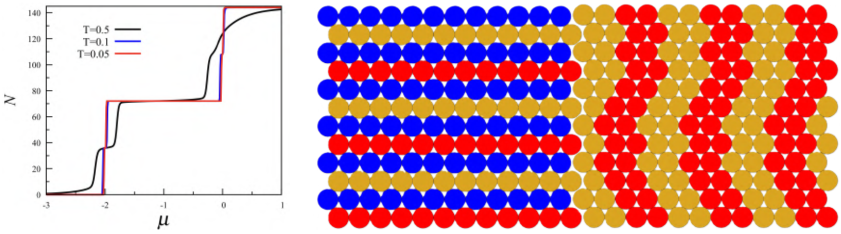


$N = 72$ $N = 144$

11. $U_{\rm AA} = U_{\rm BB} = (0, 0, 0)$, $U_{\rm AB} = (-1, 2, 1)$

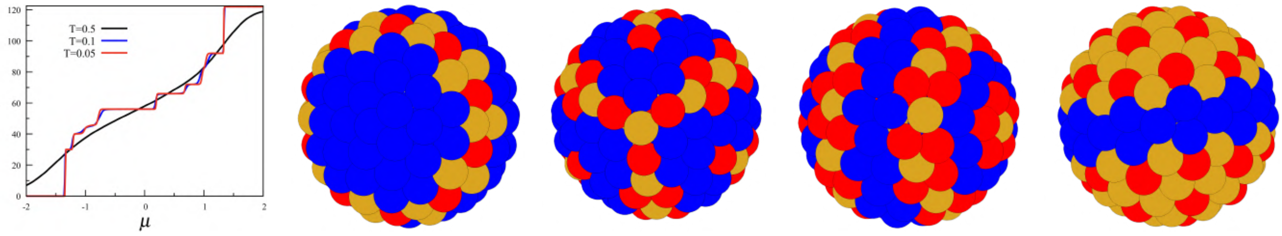


$N = 30$ $N = 56$ $N = 72$ $N = 92$

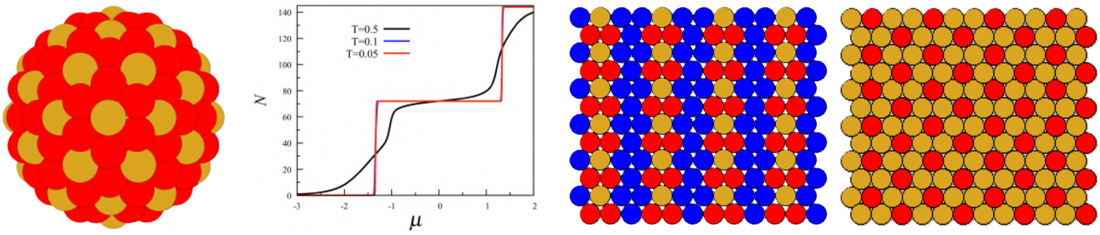


$N = 122$ $N = 72$ $N = 144$

12. $U_{\mathrm{AA}} = U_{\mathrm{BB}} = (0, 0, 0)$, $U_{\mathrm{AB}} = (-1, 1, 0)$

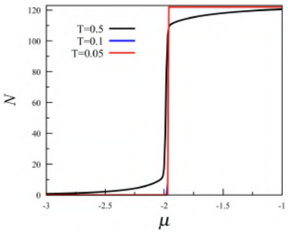


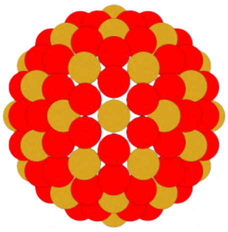

$N = 122$

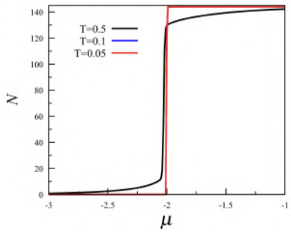


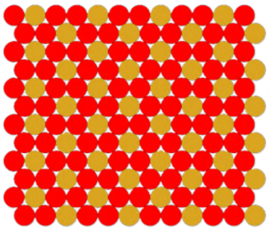

$N = 144$

13. $U_{\mathrm{AA}} = U_{\mathrm{BB}} = (0, 0, 0)$, $U_{\mathrm{AB}} = (-1, 0, 1)$

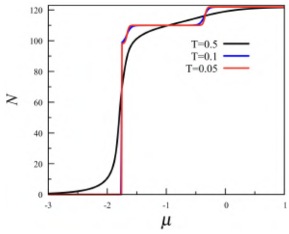


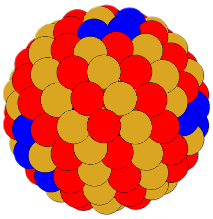

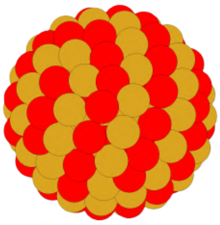

$N = 110$ $N = 122$

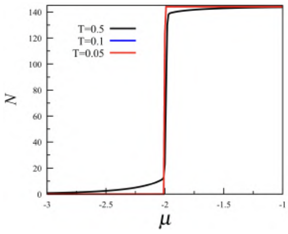


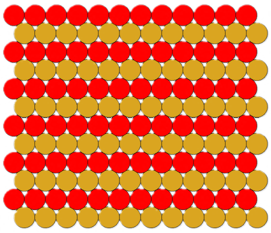

$N = 144$

14. $U_{\mathrm{AA}} = U_{\mathrm{BB}} = (1, 0, 0)$, $U_{\mathrm{AB}} = (-1, 0, 0)$

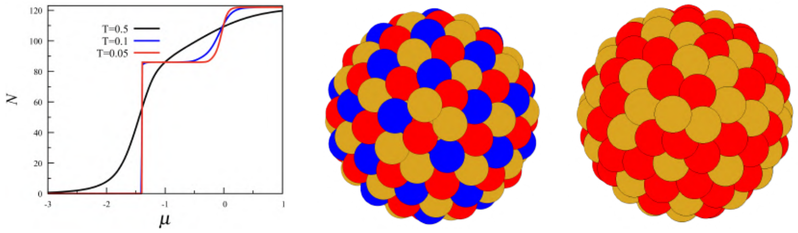


$N = 86$ $N = 122$

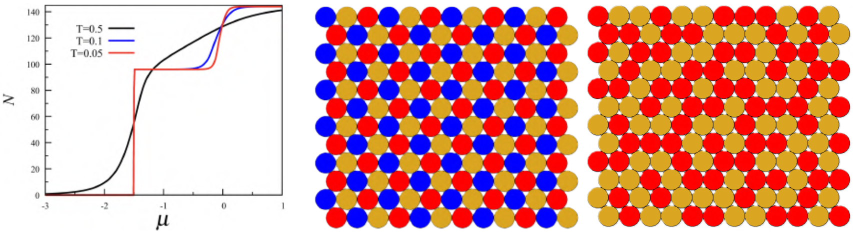


$N = 96$ $N = 144$

15. $U_{\mathrm{AA}} = U_{\mathrm{BB}} = (1, 0, 0)$, $U_{\mathrm{AB}} = (-1, -1, 0)$

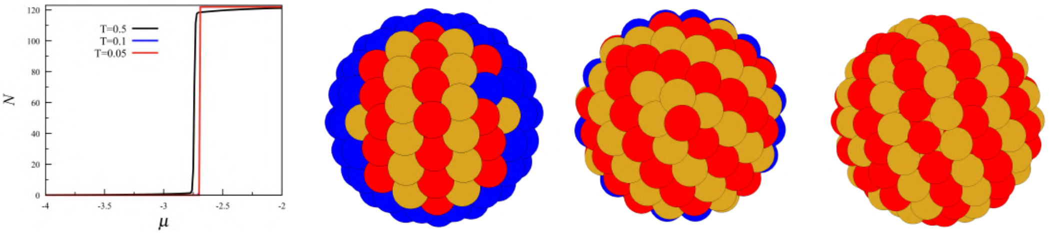


$N = 30$ $N = 60$ $N = 122$

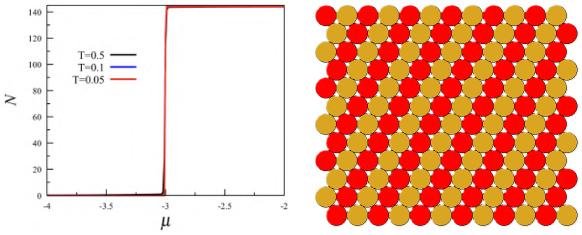


$N = 144$

16. $U_{\rm AA} = U_{\rm BB} = (1, 0, 0)$, $U_{\rm AB} = (-1, -1, -1)$

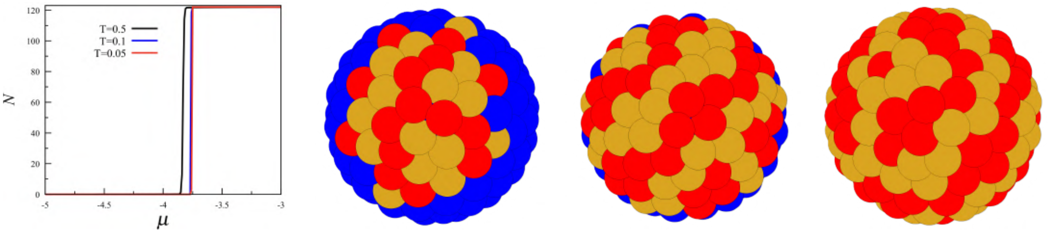


$N = 30$ $N = 60$ $N = 122$

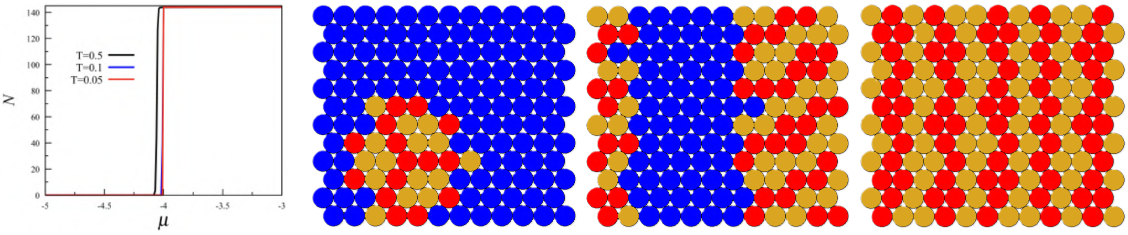


$N = 30$ $N = 80$ $N = 144$

17. $U_{\rm AA} = U_{\rm BB} = (1, 0, 0)$, $U_{\rm AB} = (1, -1, 0)$

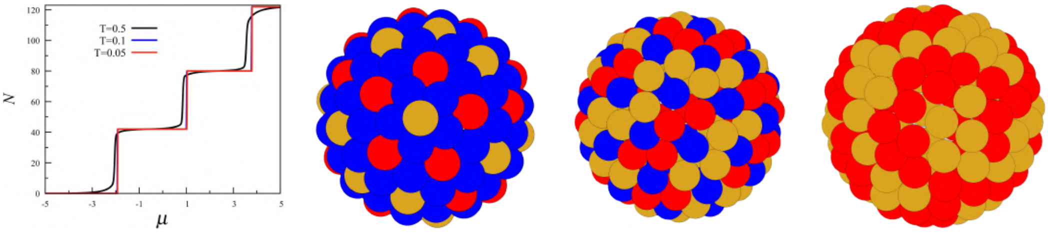


$N = 42$ $N = 80$ $N = 122$

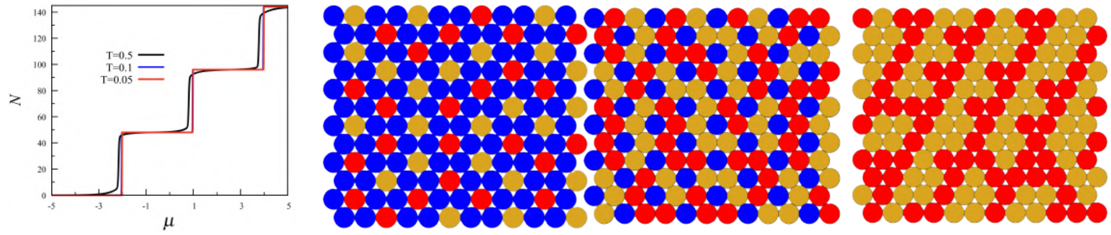


$N = 48$ $N = 96$ $N = 144$

18. $U_{\mathrm{AA}} = U_{\mathrm{BB}} = (1, 0, 0)$, $U_{\mathrm{AB}} = (1, 0, -1)$

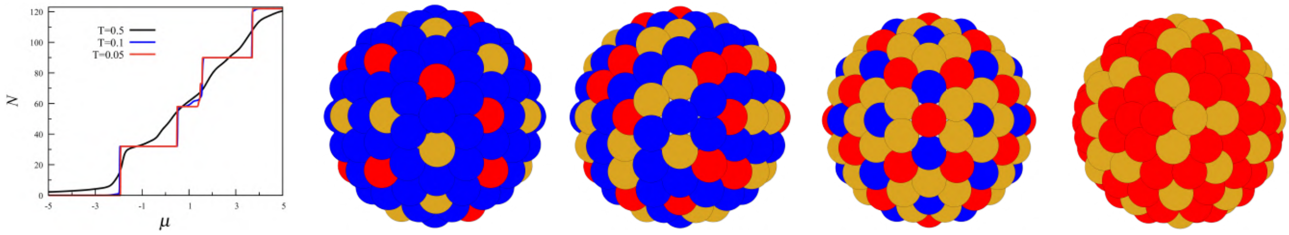


$N = 32$ $N = 58$ $N = 90$ $N = 122$

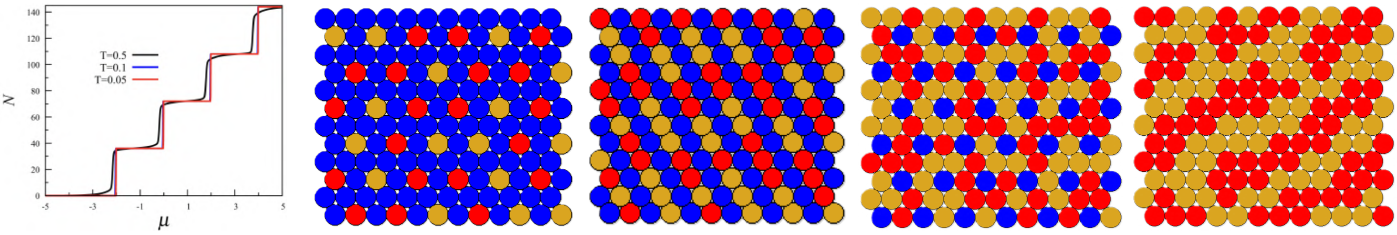


$N = 36$ $N = 72$ $N = 108$ $N = 144$

19. $U_{\mathrm{AA}} = U_{\mathrm{BB}} = (1, 0, 0)$, $U_{\mathrm{AB}} = (-1, 2, 1)$

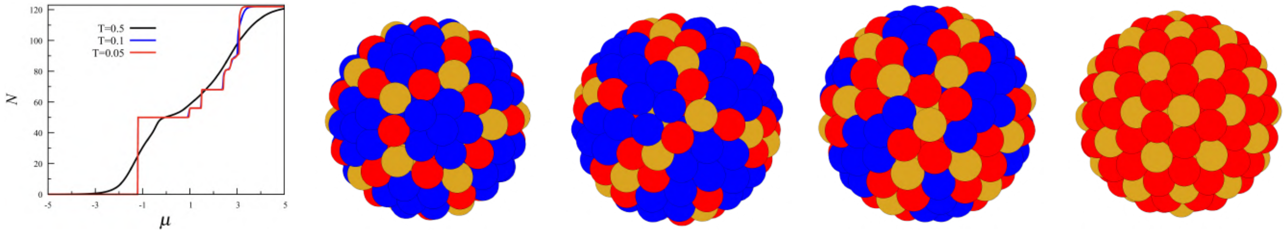


$N = 50$ $N = 56$ $N = 68$ $N = 122$

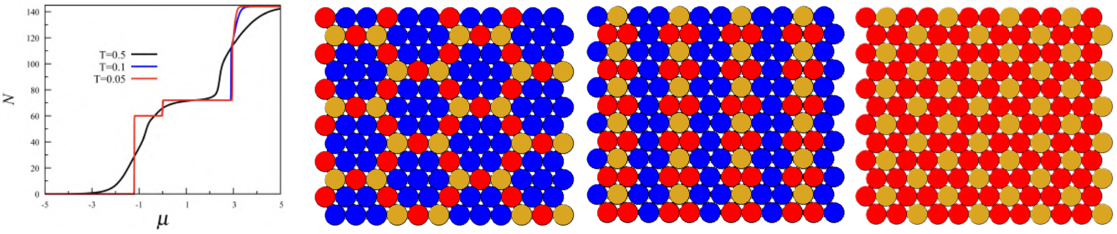


$N = 60$ $N = 72$ $N = 144$

20. $U_{\mathrm{AA}} = U_{\mathrm{BB}} = (1, 0, 0)$, $U_{\mathrm{AB}} = (-1, 1, 0)$

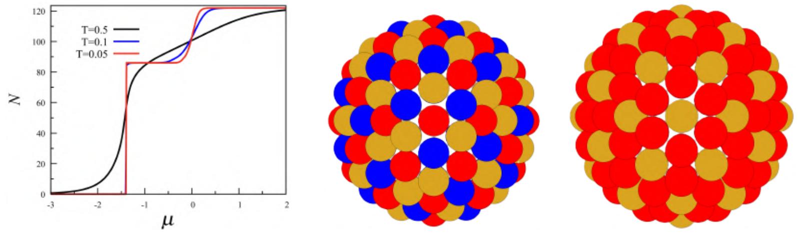


$N = 86$ $N = 122$

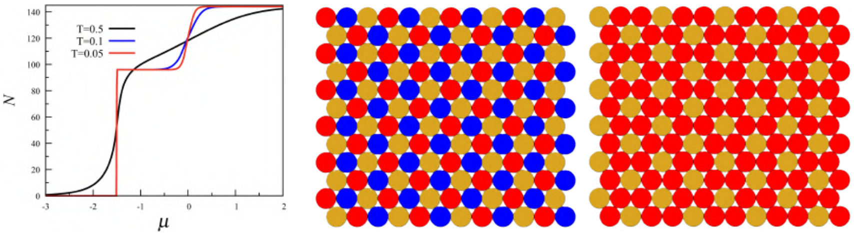


$N = 96$ $N = 144$

21. $U_{\mathrm{AA}} = U_{\mathrm{BB}} = (1, 0, 0)$, $U_{\mathrm{AB}} = (-1, 0, 1)$

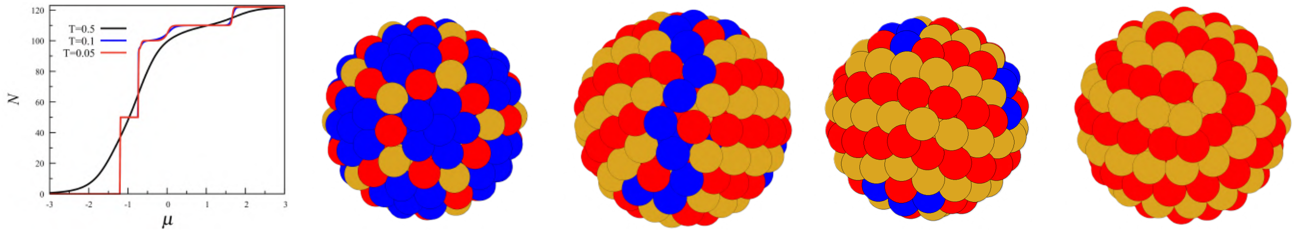


$N = 50$ $N = 100$ $N = 110$ $N = 122$

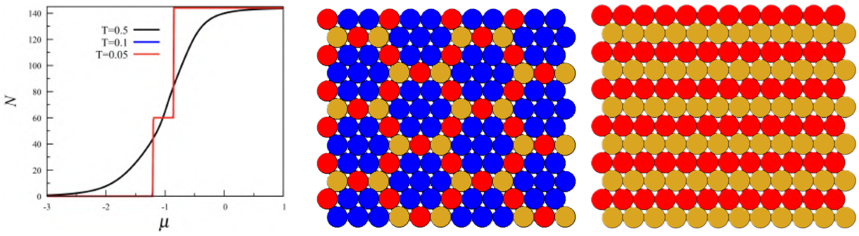


$N = 60$ $N = 144$

22. $U_{\mathrm{AA}} = U_{\mathrm{BB}} = (1,1,0)$, $U_{\mathrm{AB}} = (-1,0,0)$

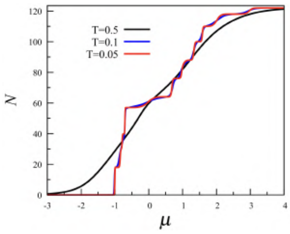


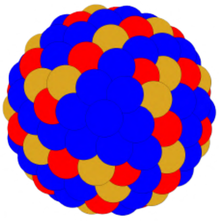

$N = 57$

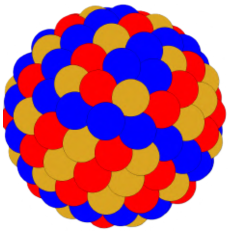

$N = 76$

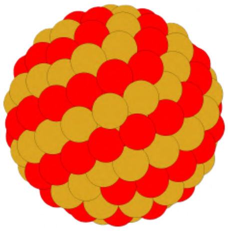

$N = 122$

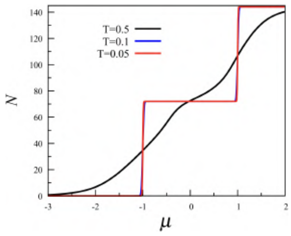


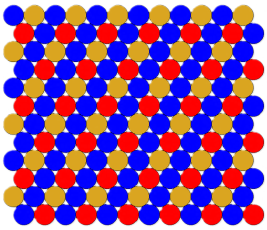

$N = 72$

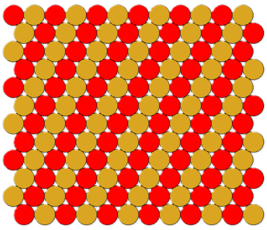

$N = 144$

23. $U_{\mathrm{AA}} = U_{\mathrm{BB}} = (1,1,0)$, $U_{\mathrm{AB}} = (-1,-1,0)$

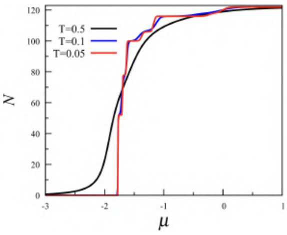


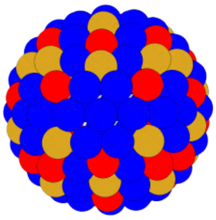

$N = 52$

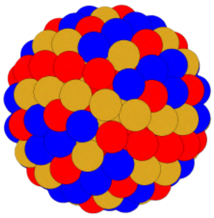

$N = 78$

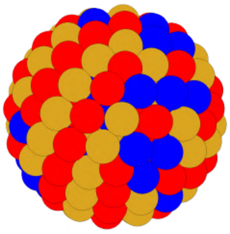

$N = 100$

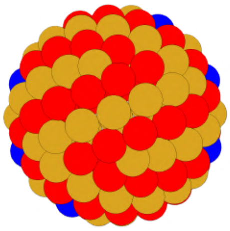

$N = 116$

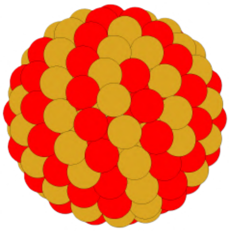

$N = 122$

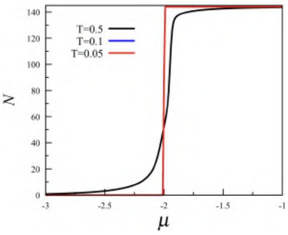


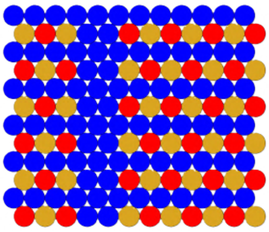

$N = 60$

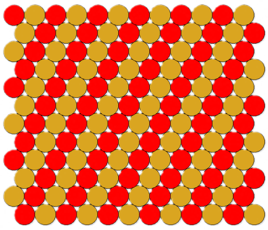

$N = 144$

24. $U_{\mathrm{AA}} = U_{\mathrm{BB}} = (1, 1, 0)$, $U_{\mathrm{AB}} = (1, -1, 0)$

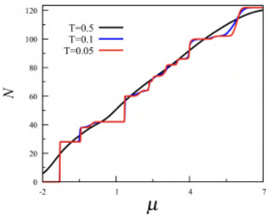


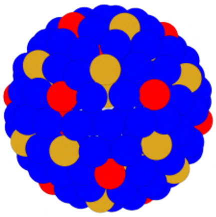

$N = 28$

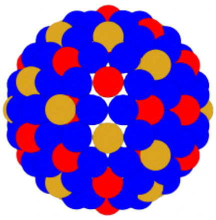

$N = 42$

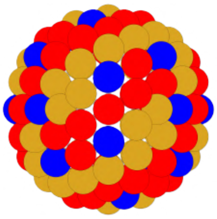

$N = 100$

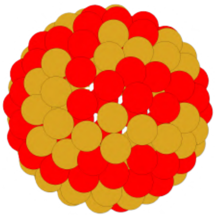

$N = 122$

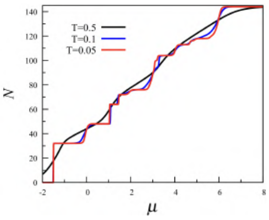


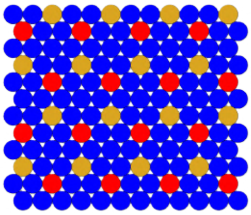

$N = 32$

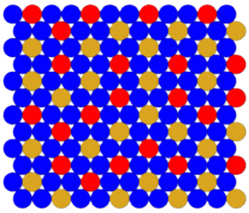

$N = 48$

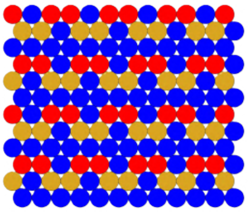

$N = 64$

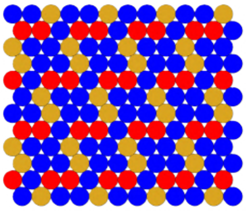

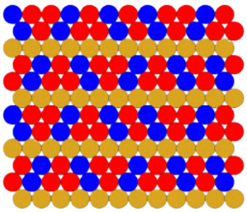

$N = 104$

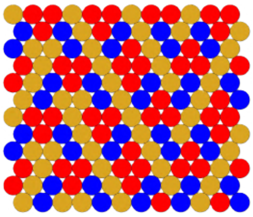

$N = 104$

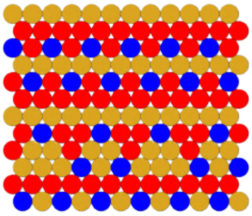

$N = 118$

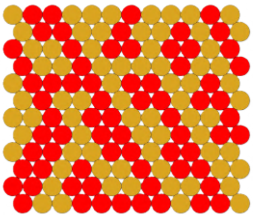

$N = 144$

25. $U_{\mathrm{AA}} = U_{\mathrm{BB}} = (1, 1, 0)$, $U_{\mathrm{AB}} = (1, 0, -1)$

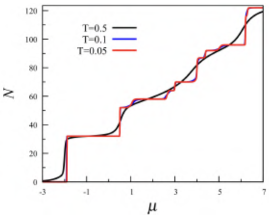


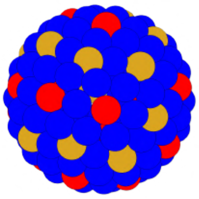

$N = 32$

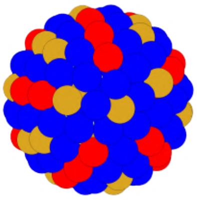

$N = 52$

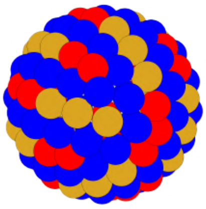

$N = 58$

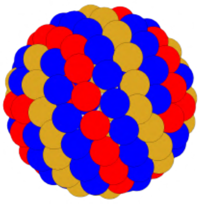

$N = 70$

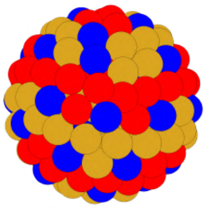

$N = 92$

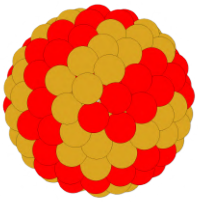

$N = 122$

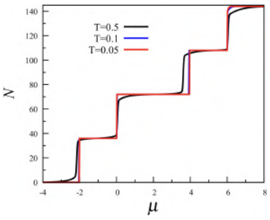


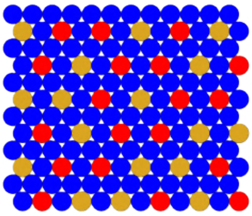

$N = 36$

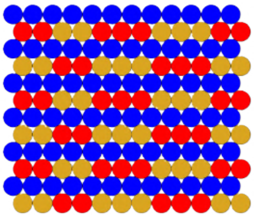

$N = 72$

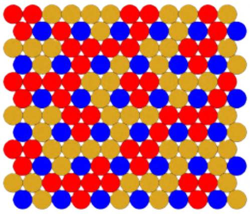

$N = 108$

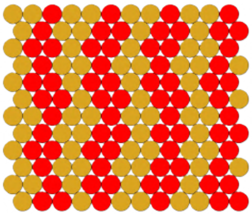

$N = 144$

26. $U_{\mathrm{AA}} = U_{\mathrm{BB}} = (1, 1, 0)$, $U_{\mathrm{AB}} = (-1, 2, 1)$

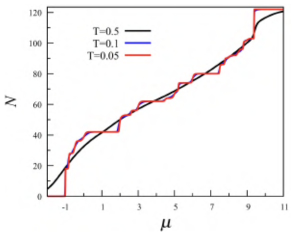


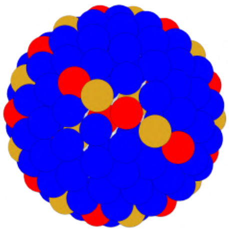
$N = 28$

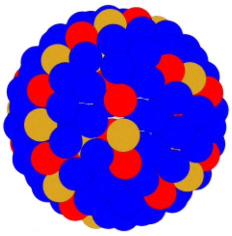
$N = 36$

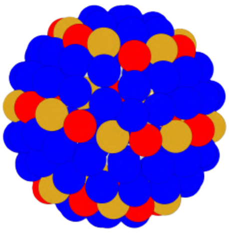
$N = 42$

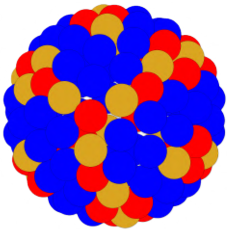
$N = 56$

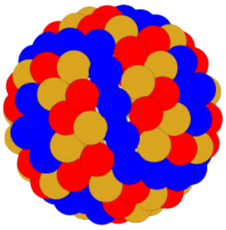
$N = 80$

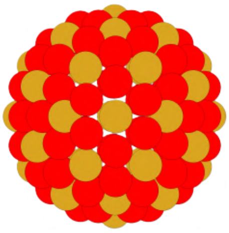
$N = 122$

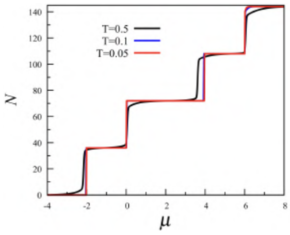


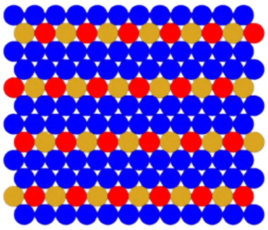
$N = 48$

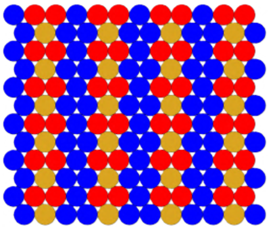
$N = 72$

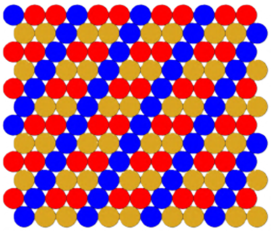
$N = 96$

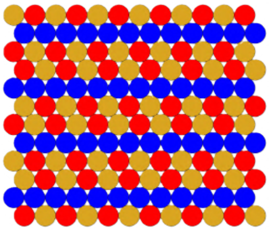
$N = 96$

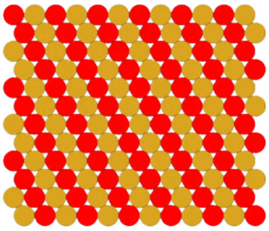
$N = 144$

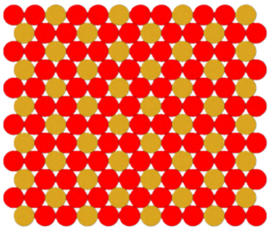
$N = 144$

27. $U_{\mathrm{AA}} = U_{\mathrm{BB}} = (1, 1, 1)$, $U_{\mathrm{AB}} = (-1, 0, 0)$

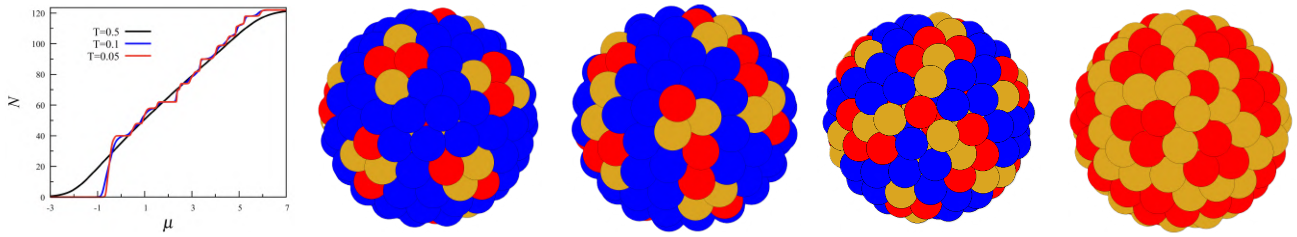


$N = 40$ $N = 48$ $N = 62$ $N = 122$

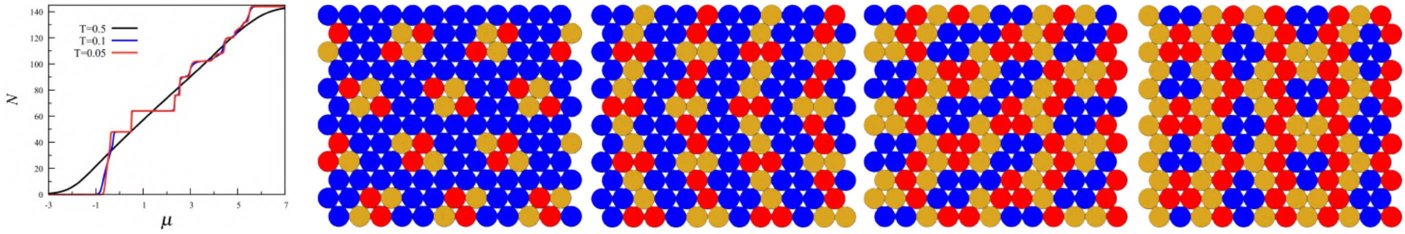


$N = 48$ $N = 64$ $N = 90$ $N = 102$

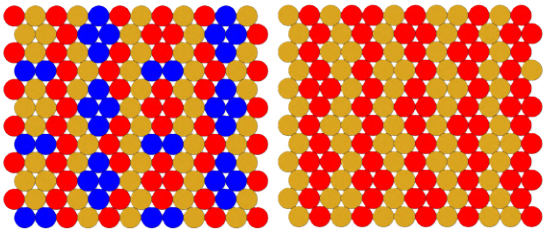

$N = 108$ $N = 144$

28. $U_{\mathrm{AA}} = U_{\mathrm{BB}} = (1, 1, 1)$, $U_{\mathrm{AB}} = (-1, -1, 0)$

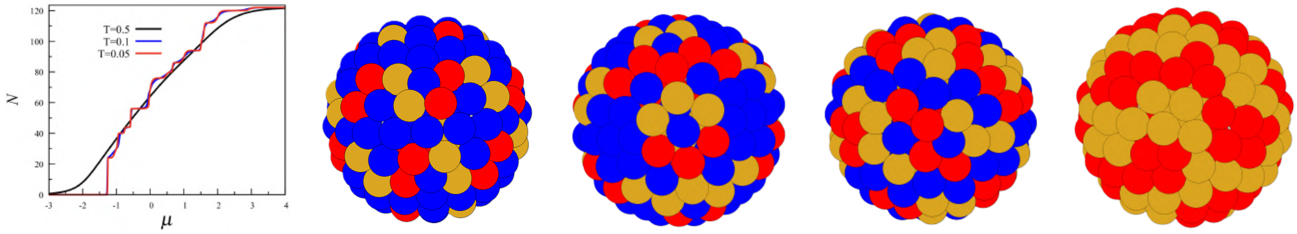


$N = 40$ $N = 56$ $N = 76$

$N = 122$

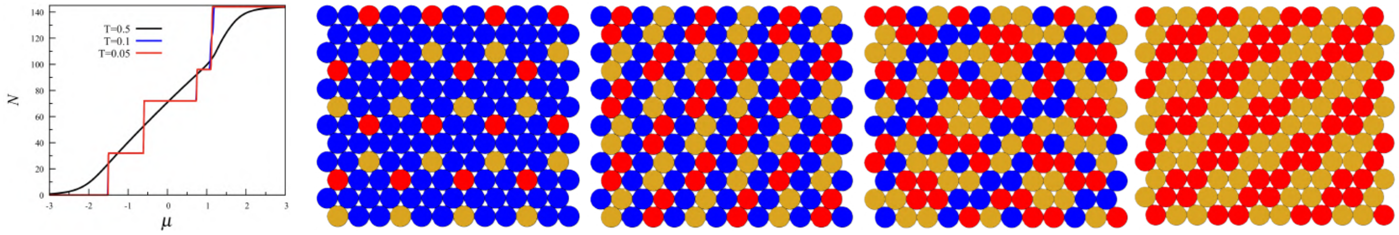


$N = 32$ $N = 72$ $N = 96$ $N = 144$

29. $U_{\mathrm{AA}} = U_{\mathrm{BB}} = (1, 1, 1)$, $U_{\mathrm{AB}} = (-1, 2, 1)$

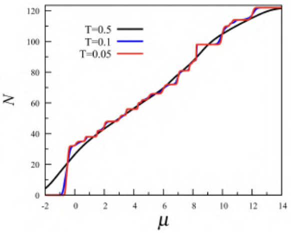


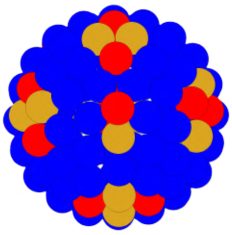

$N = 38$

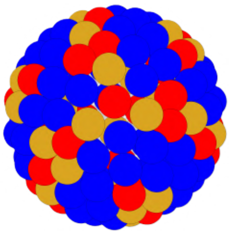

$N = 56$

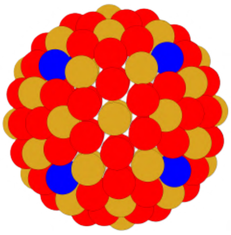

$N = 114$

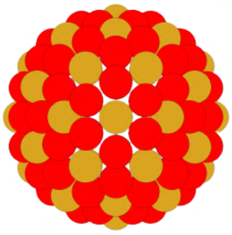

$N = 122$

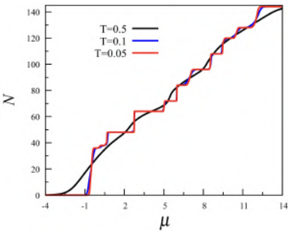


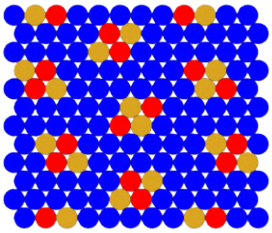

$N = 36$

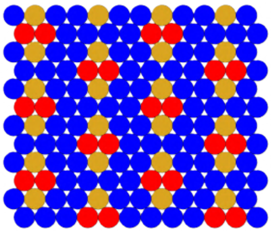

$N = 48$

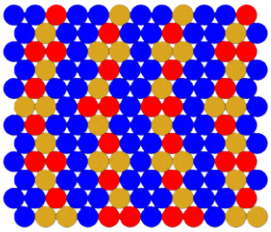

$N = 64$

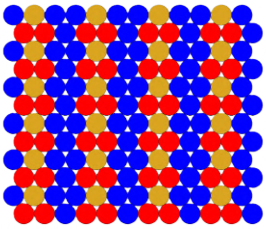

$N = 72$

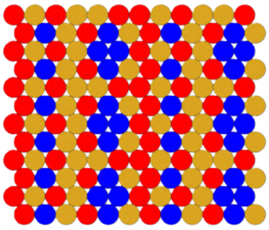

$N = 108$

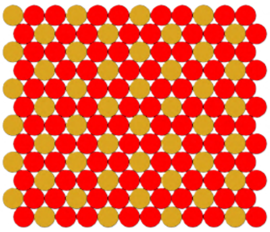

$N = 144$

30. $U_{\mathrm{AA}} = U_{\mathrm{BB}} = (-1, 0, 0)$, $U_{\mathrm{AB}} = (-1, 0, 0)$

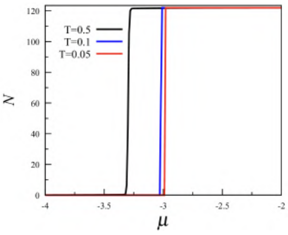


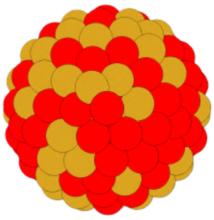

$N = 122$

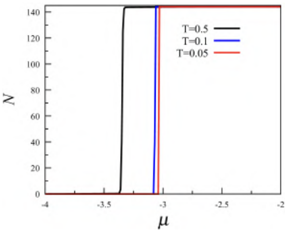


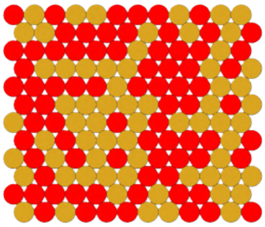

$N = 144$

31. $U_{\mathrm{AA}} = U_{\mathrm{BB}} = (-1, 0, 0)$, $U_{\mathrm{AB}} = (-1, 2, 1)$

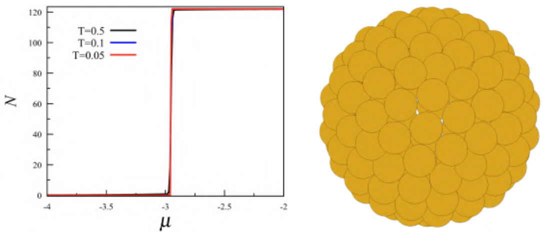


$N = 122$

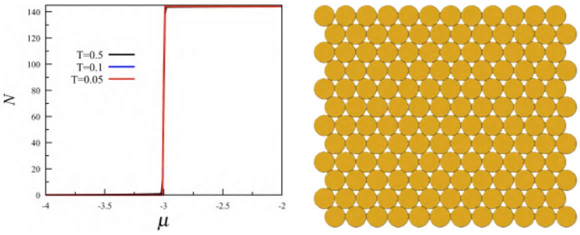


$N = 144$

32. $U_{\mathrm{AA}} = U_{\mathrm{BB}} = (1, -1, 0)$, $U_{\mathrm{AB}} = (-1, 0, 0)$

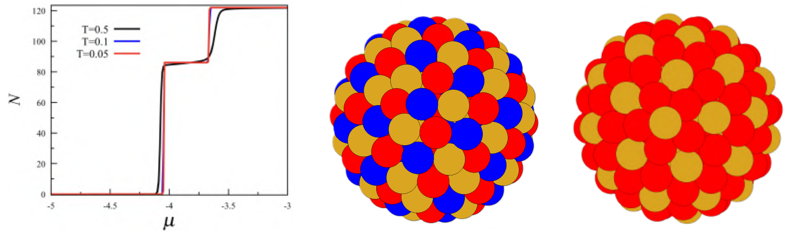


$N = 86$ $N = 122$

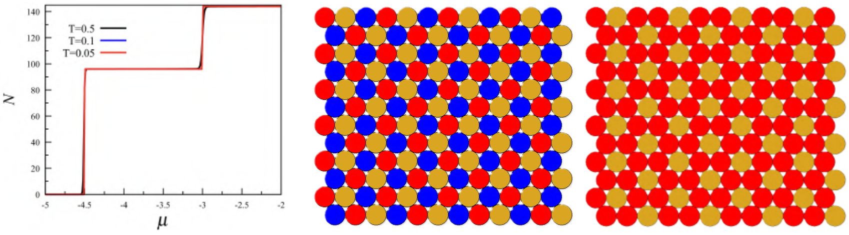


$N = 96$ $N = 144$

33. $U_{\rm AA} = U_{\rm BB} = (1, 0, -1)$, $U_{\rm AB} = (-1, 0, 0)$

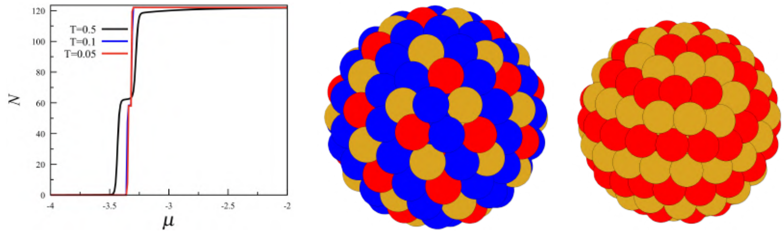


$N = 58$ $N = 122$

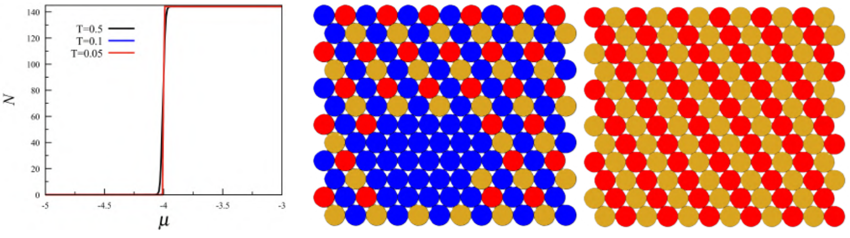


$N = 60$ $N = 144$

34. $U_{\rm AA} = U_{\rm BB} = (-1, 2, 1)$, $U_{\rm AB} = (1, 0, 0)$

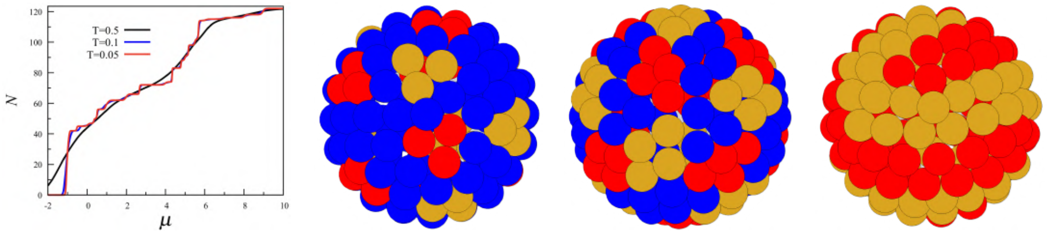


$N = 42$ $N = 72$ $N = 122$

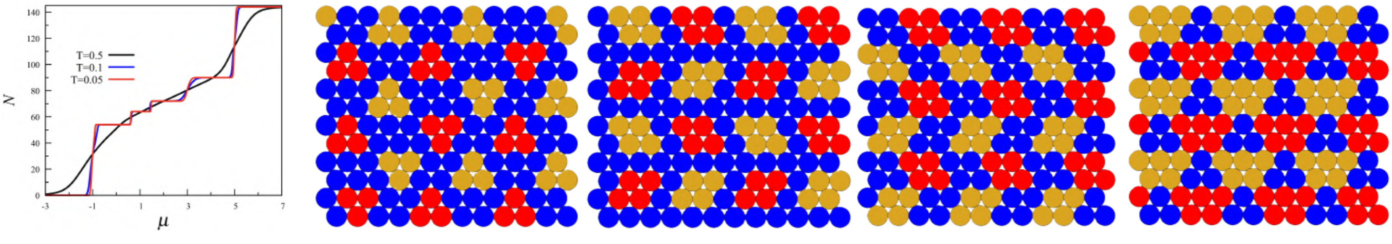


$N = 54$ $N = 64$ $N = 72$ $N = 90$

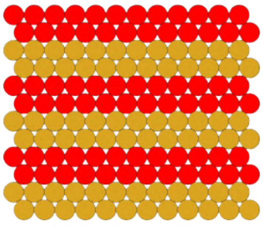

$N = 144$

35. $U_{\mathrm{AA}} = U_{\mathrm{BB}} = (-1, 2, 1)$, $U_{\mathrm{AB}} = (1, 1, 0)$

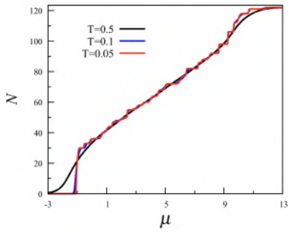


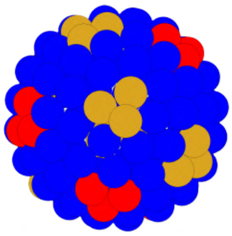

$N = 36$

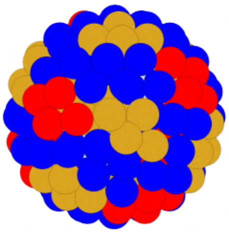

$N = 60$

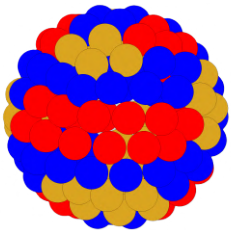

$N = 72$

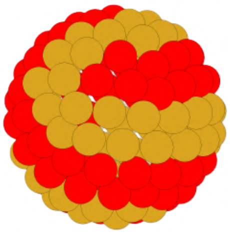

$N = 122$

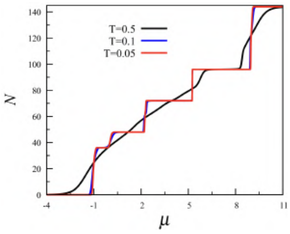


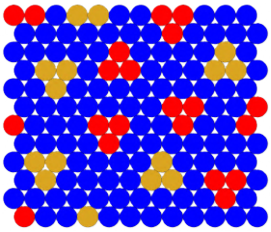

$N = 36$

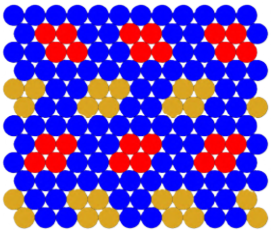

$N = 48$

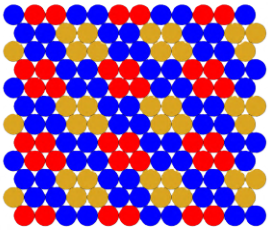

$N = 72$

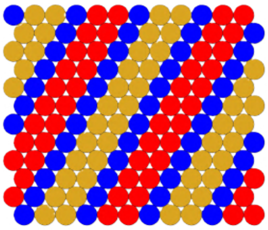

$N = 96$

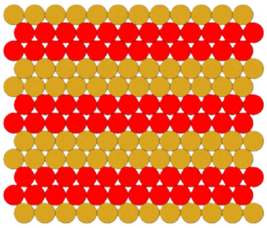

$N = 144$

36. $U_{\mathrm{AA}} = U_{\mathrm{BB}} = (-1, 2, 1)$, $U_{\mathrm{AB}} = (1, 1, 1)$

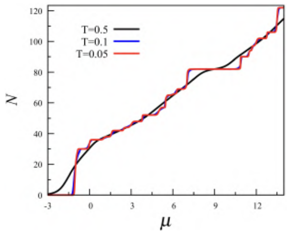


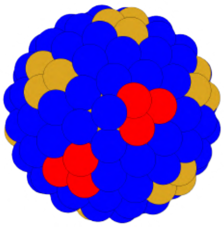

$N = 36$

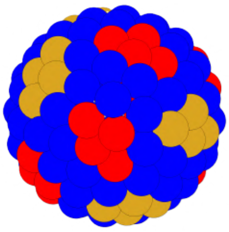

$N = 48$

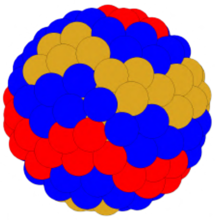

$N = 65$

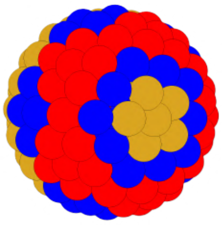

$N = 82$

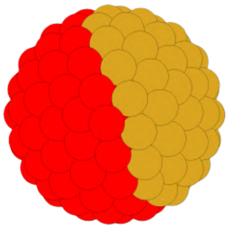

$N = 122$

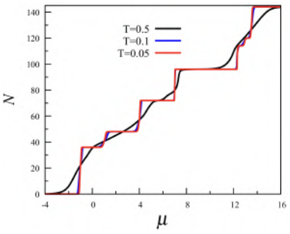


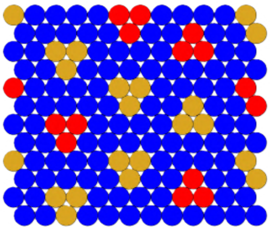

$N = 36$

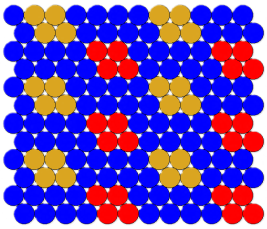

$N = 48$

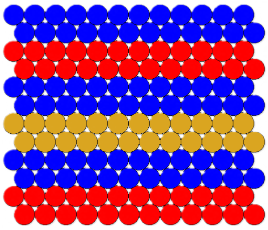

$N = 72$

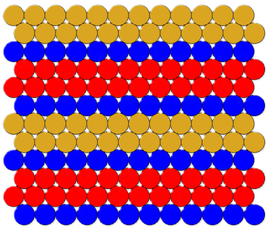

$N = 96$

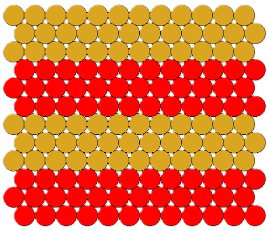

$N = 144$

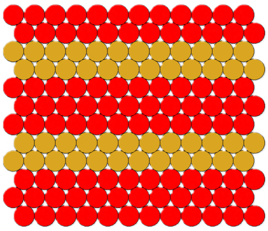

$N = 144$

37. $U_{\mathrm{AA}} = U_{\mathrm{BB}} = (-1, 2, 1)$, $U_{\mathrm{AB}} = (-1, 0, 0)$

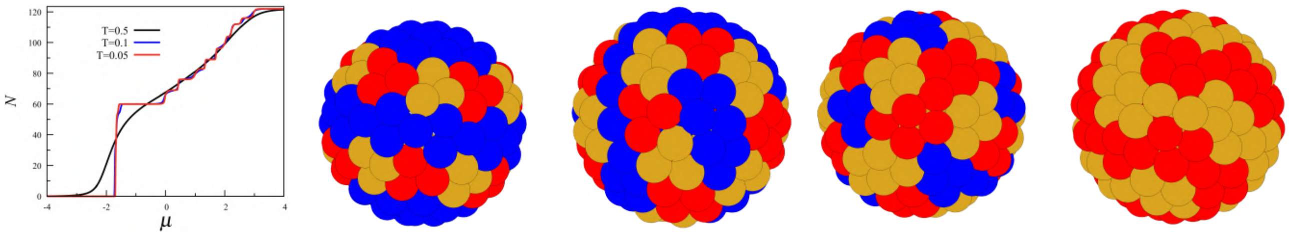


$N = 60$ $N = 76$ $N = 89$ $N = 122$

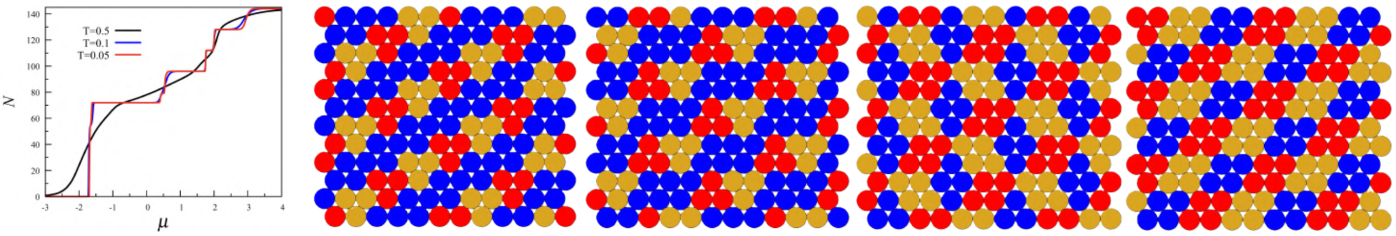


$N = 72$ $N = 72$ $N = 96$ $N = 96$

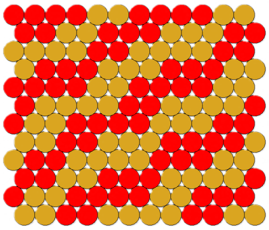

$N = 144$

38. $U_{\mathrm{AA}} = U_{\mathrm{BB}} = (-1, 2, 1)$, $U_{\mathrm{AB}} = (1, -1, 0)$

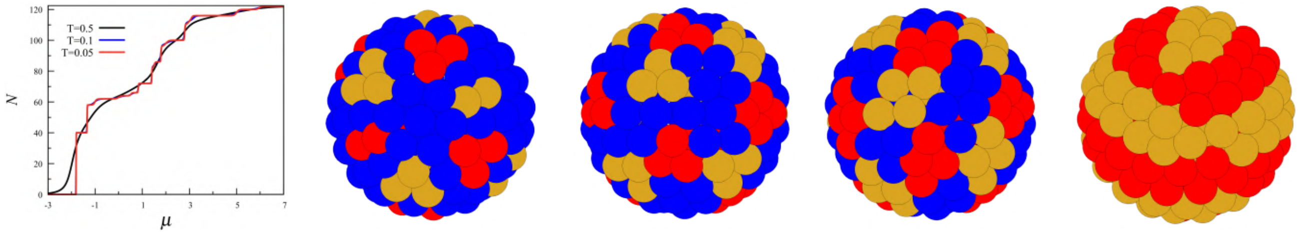


$N = 40$ $N = 58$ $N = 72$ $N = 122$

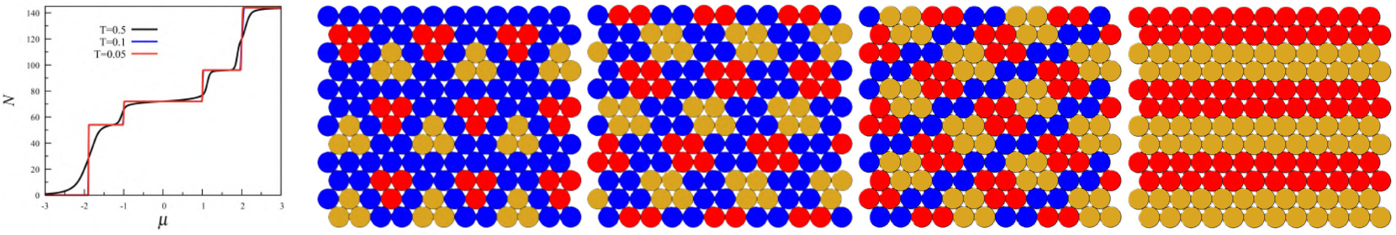


$N = 54$ $N = 72$ $N = 96$ $N = 144$

39. $U_{\mathrm{AA}} = U_{\mathrm{BB}} = (-1, 1, 0)$, $U_{\mathrm{AB}} = (1, -1, 0)$

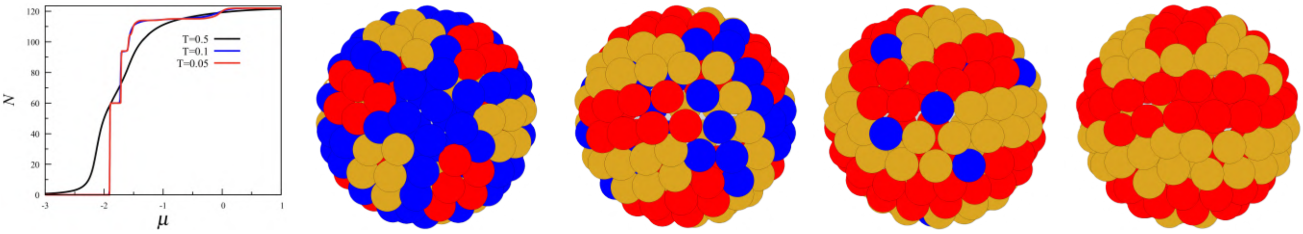


$N = 60$ $N = 94$ $N = 114$ $N = 122$

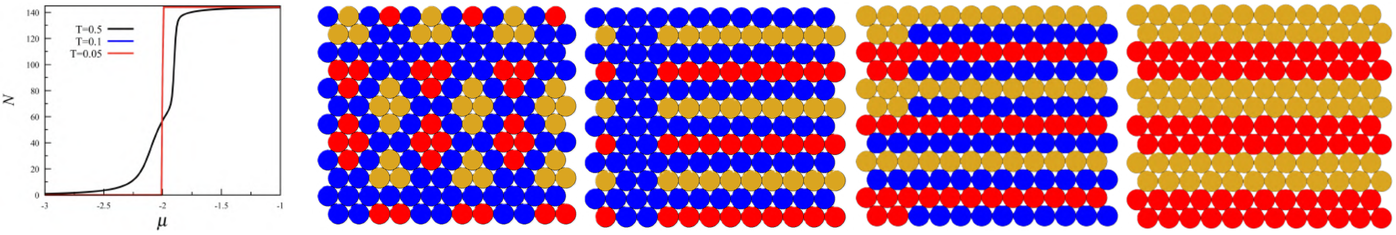


$N = 60$ $N = 60$ $N = 80$ $N = 144$

40. $U_{\mathrm{AA}} = U_{\mathrm{BB}} = (-1, 0, 1)$, $U_{\mathrm{AB}} = (1, 0, -1)$

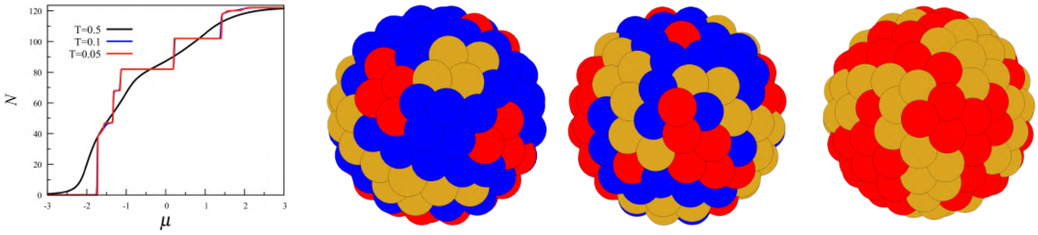


$N = 47$ $N = 82$ $N = 122$

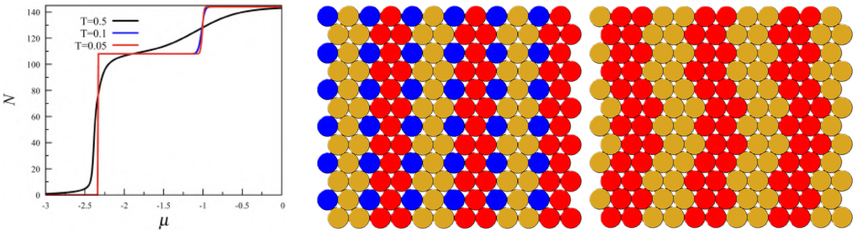


$N = 108$ $N = 144$

# 2. Asymmetric Mixtures

41. $U_{\text{AA}} = (0, 0, 0), U_{\text{BB}} = (-1, 0, 0),\ U_{\text{AB}} = (-1, 0, 0),\ N$ da 0 a 122

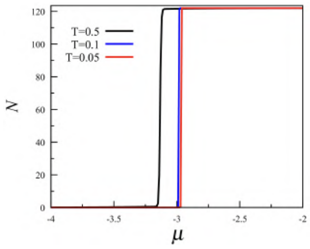


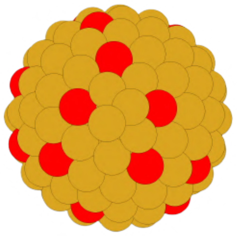

$N = 122$

42. $U_{\text{AA}} = (0, 0, 0), U_{\text{BB}} = (-1, 0, 0),\ U_{\text{AB}} = (-1, -1, 0)$

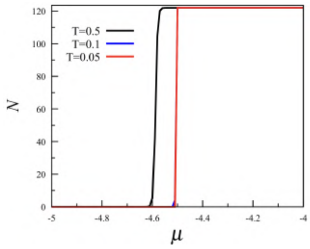


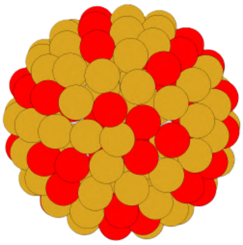

$N = 122$

43. $U_{\text{AA}} = (0, 0, 0), U_{\text{BB}} = (1, -1, 0),\ U_{\text{AB}} = (-1, 0, 0)$

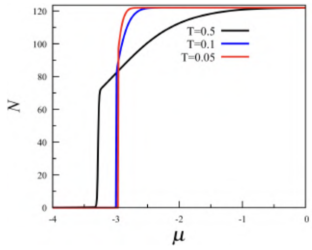


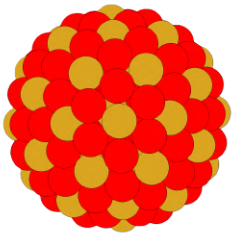

$N = 122$

44. $U_{\mathrm{AA}} = (0,0,0), U_{\mathrm{BB}} = (1,-1,0),\, U_{\mathrm{AB}} = (-1,-1,0)$

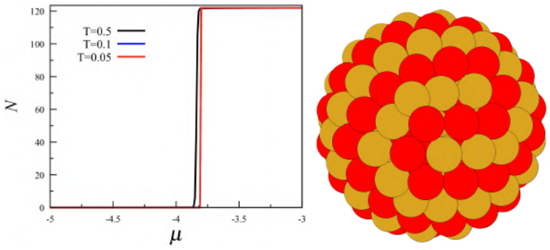


$N = 122$

45. $U_{\mathrm{AA}} = (0,0,0), U_{\mathrm{BB}} = (1,0,-1),\, U_{\mathrm{AB}} = (-1,0,0)$

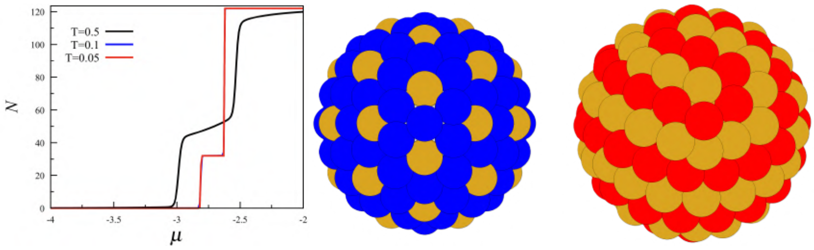


$N = 32$ $\quad$ $N = 122$

46. $U_{\mathrm{AA}} = (0,0,0), U_{\mathrm{BB}} = (1,0,-1),\, U_{\mathrm{AB}} = (-1,-1,0)$

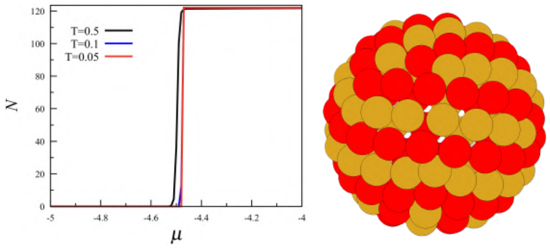


$N = 122$

47. $U_{\mathrm{AA}} = (0, 0, 0), U_{\mathrm{BB}} = (-1, 2, 1),\ U_{\mathrm{AB}} = (-1, 0, 0)$

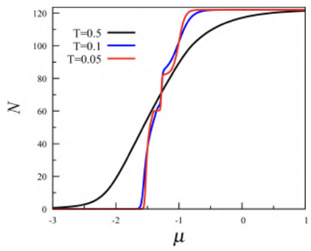


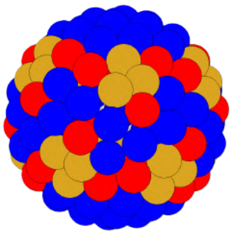

$N = 60$

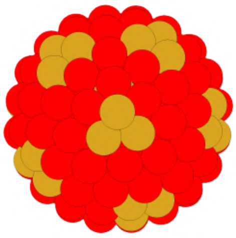

$N = 122$

48. $U_{\mathrm{AA}} = (0, 0, 0), U_{\mathrm{BB}} = (-1, 2, 1),\ U_{\mathrm{AB}} = (-1, -1, 0)$

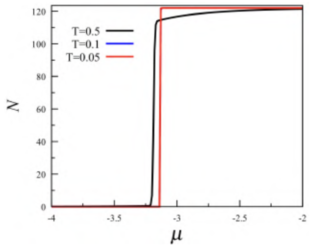


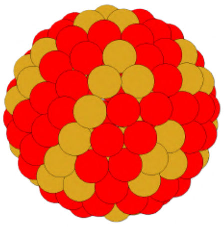

$N = 122$

49. $U_{\mathrm{AA}} = (0, 0, 0), U_{\mathrm{BB}} = (-1, 0, 1),\ U_{\mathrm{AB}} = (-1, 0, 0),\ N$ da 0 a 122

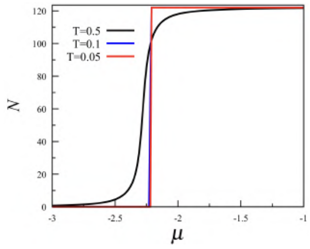


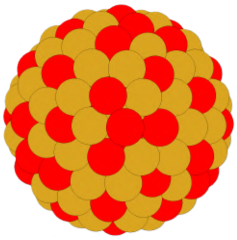

$N = 122$

50. $U_{\mathrm{AA}} = (0,0,0), U_{\mathrm{BB}} = (-1,0,1)$, $U_{\mathrm{AB}} = (-1,-1,0)$, $N$ da 0 a 122

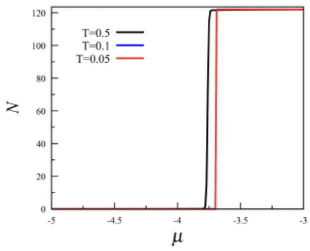


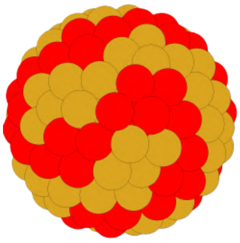

$N = 122$

# 3. Equimolar Mixtures

1. $U_{\mathrm{AA}} = U_{\mathrm{BB}} = (0,0,0)$, $U_{\mathrm{AB}} = (1,0,0)$, case 1

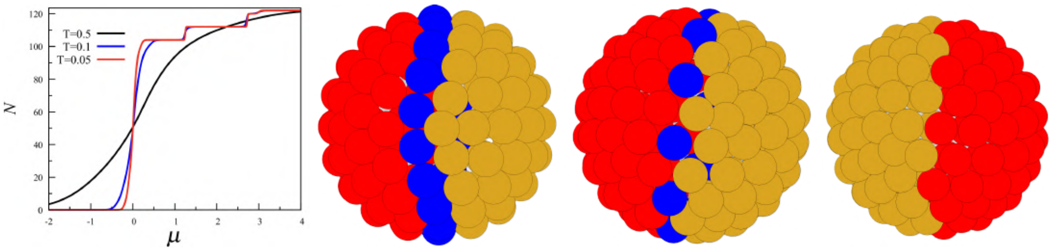


$N = 104$ $N = 112$ $N = 122$

2. $U_{\mathrm{AA}} = U_{\mathrm{BB}} = (0,0,0)$, $U_{\mathrm{AB}} = (1,1,0)$, case 2

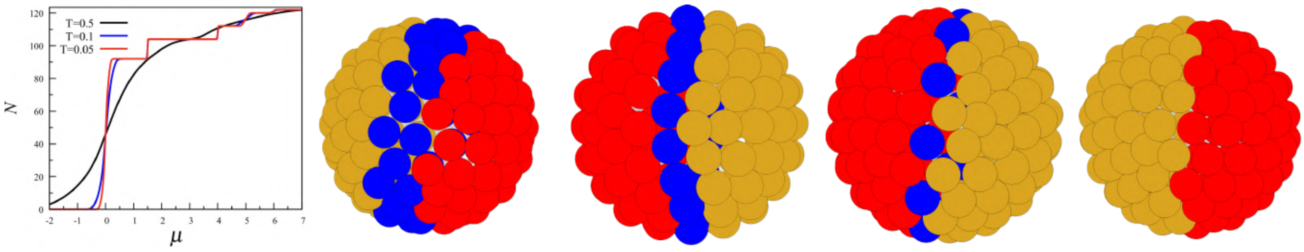


$N = 92$ $N = 104$ $N = 112$ $N = 122$

3. $U_{\mathrm{AA}} = U_{\mathrm{BB}} = (1,0,0)$, $U_{\mathrm{AB}} = (0,0,0)$, case 3

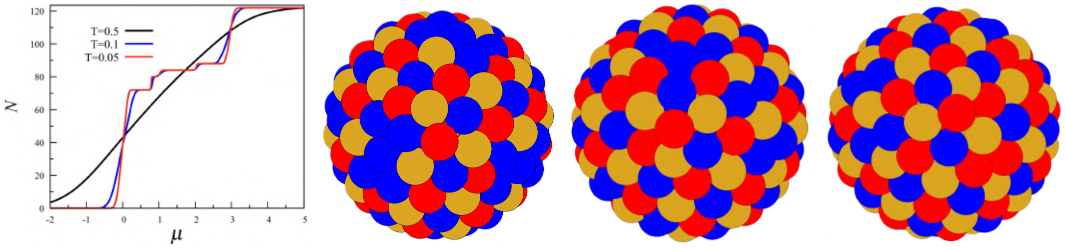


$N = 72$ $N = 80$ $N = 84$

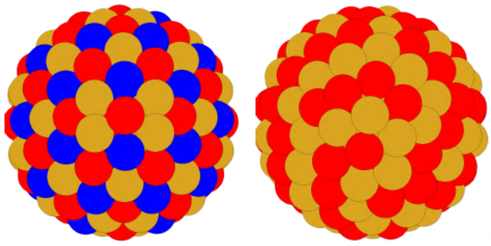

$N = 88$ $N = 122$

4. $U_{\mathrm{AA}} = U_{\mathrm{BB}} = (0,0,0)$, $U_{\mathrm{AB}} = (1,-1,0)$ , case 9

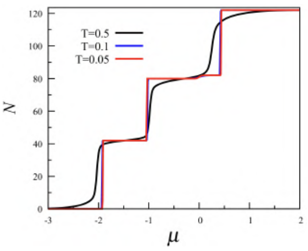


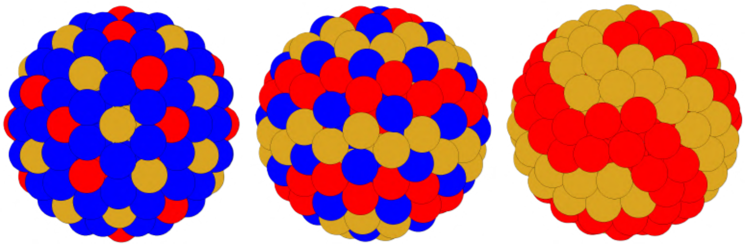

$N = 42$ $N = 80$ $N = 122$

5. $U_{\mathrm{AA}} = U_{\mathrm{BB}} = (0,0,0), U_{\mathrm{AB}} = (1,0,-1)$, case 10

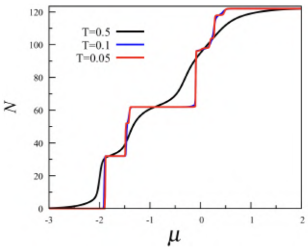


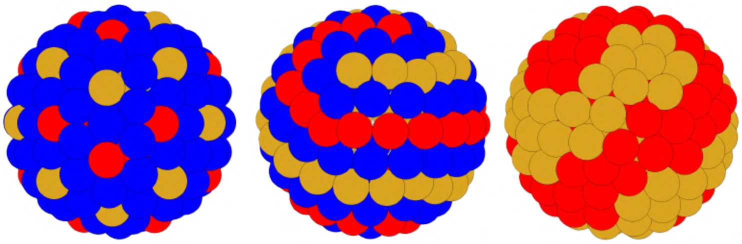

$N = 32$ $N = 62$ $N = 122$

6. $U_{\mathrm{AA}} = U_{\mathrm{BB}} = (1,0,0)$, $U_{\mathrm{AB}} = (1,0,-1)$, case 18

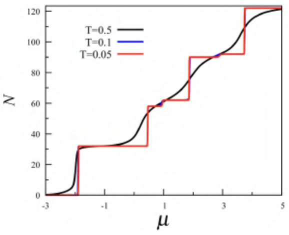


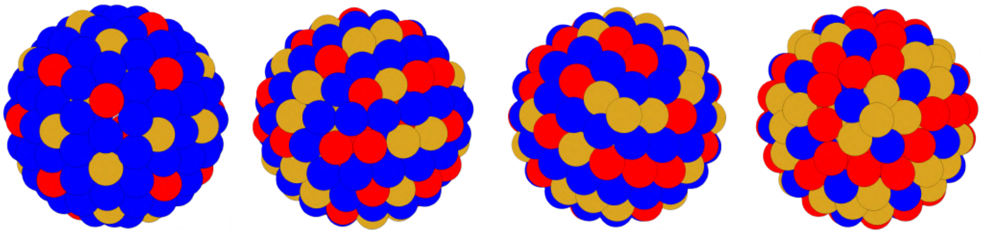

$N = 58$ $N = 58$ $N = 62$ $N = 90$

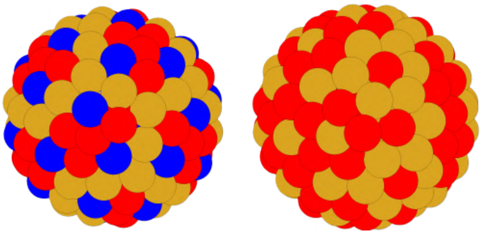

$N = 92$ $N = 122$
